# Supplementary material for: Geometric Model Checking of Continuous Space
Source: arXiv:2105.06194 source file (2022-11-21)
Supplement: Supplementary file 1 [file appendix-b.tex]

\section{Algorithms, pseudo-code, correctness, complexity}
\label{sec:appendix-b}
Currently \PolyLogicA represents a polyhedral model $\model{X}$ through an explicit encoding of the Kripke model from Definition~\ref{def:KrpS}.
The latter is stored as a graph having the simplexes as nodes and with $\face$ as the edge relation.
The current implementation stores the out-neighborhood $\OUT(\sigma) = \{\tau \,|\, \sigma \face \tau\}$ and the in-neighborhood $\IN(\sigma) = \{\tau \,|\, \sigma \facer \tau\}$ of each node $\sigma$ in two separate arrays, allowing access in constant time to these sets.

In what follows, we indicate with $n$ the number of simplexes and with $d$ the dimension of $\Ksc$, that is, the maximum dimension of a simplex in $\Ksc$.
Indeed, the number of nodes of the encoding is $n$.
Moreover, since each simplex $\sigma$ has at most $d$ vertices and the faces of $\sigma$ are generated by subsets of vertices, the cardinality of each out-neighborhood is at most $2^{d}$, and so the total number of edges is at most $n\cdot 2^{d}$.
We let $N$ be the total size $N$ of the Kripke structure (sum of the number of nodes and edges), which is therefore in $\mathcal{O}(n \cdot 2^{d+1})$.

The semantics of the reachability operator, as of Definition~\ref{def:kripke-semantics}, is computed via a variant of the flooding procedure already employed in~\cite{CLLM16,CGLLM15,Gri16}, retaining its asymptotic complexity (linear in $N$). 
The pseudo-code is reported in Figure~\ref{fig:pseudo-code}. Therein, for brevity, we call ``good'' a $\pm$-path witnessing the formula $\GL(\phi,\psi)$.

\begin{figure}
\begin{lstlisting}[
    escapeinside={(*}{*)},
    basicstyle=\scriptsize,
    breaklines=true,
    postbreak=\mbox{$\hookrightarrow$\space},
    numbers=left,
    xleftmargin=2em,
    framexleftmargin=1.5em
]
    Input:  (*$\semKM{\phi}, \semKM{\psi}$*) sets of nodes of a reflexive, transitive graph
    Output: (*$\semKM{\GL(\phi,\psi)}$*)
    
    // frontier: the points queued for the next iteration. Initialized with the next to last points of a good path.
    let frontier = (*$\semKM{\phi} \cap\OUT(\semKM{\psi})$*)
    
    // flooded: all the points that are in the middle of a good path.
    let flooded = frontier
    
    while frontier(*$\ne\emptyset$*):
        let (*$\sigma$*) = frontier.pop()
        for every (*$\tau \in \IN(\sigma) \cup \OUT(\sigma)$*):
            if (*$\tau \notin$*)flooded and (*$\tau \in \semKM{\phi}$*):
                frontier.add((*$\tau$*))
                flooded.add((*$\tau$*))
    
    // result: the starting points of a good path.
    let result = (*$\IN($*)flooded(*$)$*)
    
    return result
\end{lstlisting}
\caption{\label{fig:pseudo-code}Pseudo-code for model checking the reachability operator.}
\end{figure}

\noindent
We provide a short proof of the correctness of the algorithm.

\begin{proof}[Correctness, sketch]
To be consistent with the comments in the pseudo-code, we keep calling a $\pm$-path $\pi:\{0,\dots,k\} \to \Ksc$ witnessing the satisfaction of $\GL(\phi,\psi)$ a ``good'' path.
First, notice that we can divide a good path in three parts:
the initial point $\pi(0)$, the central segment $\pi(\{1,\dots,k-1\})$ satisfying $\phi$ and the final point $\pi(k)$ satisfying $\psi$.
To compute the set $\semKM{\GL(\phi,\psi)}$ we work ``backwards''.
First, we compute the set $C := \semKM{\phi} \cap \OUT(\semKM{\psi})$ (the simplexes of the form $\pi(k-1)$ for some good path $\pi$). Then we use a standard flooding procedure to collect the nodes of the graph  that are connected to $C$ via a non-directed path passing only through $\semKM{\phi}$ (these are the simplexes of the form $\pi(1)$ for some good path $\pi$). Finally we compute the set $\semKM{\GL(\phi,\psi)} = \mbox{${\IN}(D)$}$ (the simplices of the form $\pi(0)$ for some good path $\pi$).

The code is divided in three parts, following the three steps described above:
\emph{initialization} (lines 4-8), \emph{flooding} (lines 10-15) and \emph{finalization} (lines 17-20).
In the \emph{initialization} we define the sets of simplexes \texttt{frontier} and \texttt{flooded}, which will be later used by the flooding procedure.
Both sets are initialized using $C = \semKM{\phi} \cap \OUT(\semKM{\psi})$.
The \emph{flooding} part is quite standard; it is used to compute $D$ starting from $C$.
At the end of this step, the value of $D$ is stored in the variable \texttt{flooded}.
Finally, in the \emph{finalization} we return the set $\IN(\texttt{flooded}) = \semKM{\GL(\phi,\psi)}$, which is the desired output of the algorithm.
\end{proof}

\noindent
The complexity of the implementation of the pseudo-code above in \PolyLogicA is $\mathcal{O}(N)$---notice that all the set-theoretic operations and the flooding procedure are linear in the number of nodes and edges.
The computation of the Boolean operators are also linear in $N$.
Therefore, the asymptotic complexity of the currently implemented model checking algorithm is in $\mathcal{O}(N\cdot h)$, where $h$ is the number of subformulas of the formula to be checked.
Once $d$ is fixed (as in the case of 3D meshes, where the ``exponential'' contribution of $d$ is negligible), this becomes $\mathcal{O}(n \cdot h)$.

Next, we spend some words on the complexity of the encoding, which is also part of our tool.
In the current prototype, the input is described by a list of $n$ simplexes with maximum dimension $d$, each one being represented by a list of vertices.
To compute the Kripke frame of Definition~\ref{def:KrpS} from this description, the tool performs an explicit enumeration of the subsets of each simplex, building the arrays of out- and in-neighborhood incrementally.
This results in a time complexity in $\mathcal{O}(N)$, which becomes $\mathcal{O}(n)$ once the dimension is fixed.
Therefore, for $d$ fixed, the total complexity (encoding plus model checking) is in $\mathcal{O}(n \cdot h)$.
